# Supplementary material for: Recurrent Neural Networks Learn to Store and Generate Sequences using Non-Linear Representations
Source: arXiv:2408.10920 source file (2024-08-20)
Supplement: Supplementary file 1 [file appendixTables.tex]

\begin{table*}[tp]
\centering
\setlength{\tabcolsep}{0.5em} 
%\resizebox{1\linewidth}{!}{
\begin{tabular}{l *5}{c} }
\toprule
Decoder & $N=64$ & $N=128$ & $N=256$ & $N=512$ & $N=1024$ \\
\midrule
 Autoregressive & 0.97 $\pm$ 0.00 & 1.00 $\pm$ 0.00 & 1.00 $\pm$ 0.00 & 1.00 $\pm$ 0.00 & 1.00 $\pm$ 0.00 \\
 No input & 1.00 $\pm$ 0.00 & 1.00 $\pm$ 0.00 & 1.00 $\pm$ 0.00 & 1.00 $\pm$ 0.00 & 1.00 $\pm$ 0.00 \\

\bottomrule
\end{tabular}
%}
\caption{Repeat task results. The two decoder variants refer to how the repeat phase is conducted after the model has processed the input. For the `Autoregressive' variant, the model generates tokens conditional on the tokens it has already generated. For the `No input' variant, it receives only pad tokens during generation. Both variants solve the task, but we show that they learn different solutions.}
\label{tab:evals}
\end{table*}

\begin{table*}[tp]
\centering
\setlength{\tabcolsep}{0.5em}
\resizebox{1\linewidth}{!}{
\begin{tabular}{ll *{5}{c} }
\toprule
Intervention & Variant & $N=64$ & $N=128$ & $N=256$ & $N=512$ & $N=1024$ \\
\midrule
\multirow{2}{*}{Unigram} & Autoregressive & 0.00 $\pm$ 0.00 & 0.01 $\pm$ 0.00 & 0.18 $\pm$ 0.03 & 0.91 $\pm$ 0.08 & 1.00 $\pm$ 0.00 \\
 & No input & 0.37 $\pm$ 0.17 & 1.00 $\pm$ 0.00 & 1.00 $\pm$ 0.00 & 1.00 $\pm$ 0.00 & 1.00 $\pm$ 0.01 \\
\midrule
\multirow{2}{*}{Bigram} & Autoregressive & 0.01 $\pm$ 0.00 & 0.54 $\pm$ 0.05 & 0.97 $\pm$ 0.05 & 1.00 $\pm$ 0.00 & 1.00 $\pm$ 0.00 \\
 & No input & 0.95 $\pm$ 0.06 & 1.00 $\pm$ 0.00 & 1.00 $\pm$ 0.00 & 1.00 $\pm$ 0.00 & 1.00 $\pm$ 0.00 \\
\midrule
\multirow{2}{*}{Gödel} & Autoregressive & 0.87 $\pm$ 0.03 & 0.89 $\pm$ 0.04 & 0.91 $\pm$ 0.08 & 0.95 $\pm$ 0.01 & 0.94 $\pm$ 0.04 \\
 & No input & 0.41 $\pm$ 0.04 & 0.76 $\pm$ 0.01 & 0.92 $\pm$ 0.01 & 0.96 $\pm$ 0.01 & 0.98 $\pm$ 0.00 \\
\bottomrule
\end{tabular}
}
\caption{Intervention accuracy}
\label{tab:intervention-accuracy}
\end{table*}
